# Supplementary material for: No Regret Sample Selection with Noisy Labels
Source: arXiv:2003.03179 source file (2021-04-04)
Supplement: Supplementary file 1 [file supplementary.tex]

\documentclass[10pt,twocolumn,letterpaper]{article}
\pdfoutput=1

% ICCV
\usepackage{iccv}
\usepackage{times}
\usepackage{epsfig}
\usepackage{graphicx}
\usepackage{amsmath}
\usepackage{amssymb}

% Ours
\usepackage[flushleft]{threeparttable}
\usepackage{colortbl}
\usepackage{cite}
\usepackage{amsfonts}
\usepackage{amsthm}
\usepackage{algorithm,algpseudocode}
\usepackage{multirow}
\usepackage{enumitem}
\usepackage{textcomp}
\usepackage{subcaption}
\usepackage{xcolor}
\usepackage{bm}

% Include other packages here, before hyperref.

% If you comment hyperref and then uncomment it, you should delete
% egpaper.aux before re-running latex.  (Or just hit 'q' on the first latex
% run, let it finish, and you should be clear).
\usepackage[pagebackref=true,breaklinks=true,letterpaper=true,colorlinks,bookmarks=false]{hyperref}

% \iccvfinalcopy % *** Uncomment this line for the final submission

 % *** Enter the ICCV Paper ID here

% Pages are numbered in submission mode, and unnumbered in camera-ready
\ificcvfinal\pagestyle{empty}\fi

% Algorithm
\algrenewcommand\algorithmicindent{1.0em}
\algnewcommand{\Inputs}[1]{%
  \State \textbf{Inputs:}
  \Statex \hspace*{\algorithmicindent}\parbox[t]{.8\linewidth}{\raggedright #1}
}
\algnewcommand{\Outputs}[1]{%
  \State \textbf{Outputs:}
  \Statex \hspace*{\algorithmicindent}\parbox[t]{.8\linewidth}{\raggedright #1}
}
\algnewcommand{\Initialize}[1]{%
  \State \textbf{Initialize:}
  \Statex \hspace*{\algorithmicindent}\parbox[t]{1.2\linewidth}{\raggedright #1}
}

% Theory

% Ours

\definecolor{Gray}{gray}{0.9}

\begin{document}

%%%%%%%%% TITLE
\title{Supplementary Material of ``No Regret Sample Selection with Noisy Labels''}

\author{First Author\\
Institution1\\
Institution1 address\\
{\tt\small firstauthor@i1.org}
% For a paper whose authors are all at the same institution,
% omit the following lines up until the closing ``}''.
% Additional authors and addresses can be added with ``\and'',
% just like the second author.
% To save space, use either the email address or home page, not both
\and
Second Author\\
Institution2\\
First line of institution2 address\\
{\tt\small secondauthor@i2.org}
}

\maketitle
% Remove page # from the first page of camera-ready.
\ificcvfinal\thispagestyle{empty}\fi

%%%%%%%%% BODY TEXT
\appendix
\input{texts/appendix}

{\small
\bibliographystyle{ieee_fullname}
\bibliography{egbib}
}

\end{document}
